# Supplementary material for: Practical and Asymptotically Exact Conditional Sampling in Diffusion Models
Source: arXiv:2306.17775 source file (2024-11-23)
Supplement: Supplementary file 1 [file smc_appendix.tex]

\section{Sequential Monte Carlo details}\label{sec:SMC_details}

% Original text: 
%However, for SMC to be practical the weights must be regular. Othewise when only a small fraction of particles receive nontrivial weights, the rest will be discarded and the procedure provides a poor approximation of the target distributions. See \Cref{sec:SMC_details} for details.  

%The number of particles needed for accurate estimation of each $\target_t$ is exponential in the KL divergence between successive targets \citep{chatterjee2018sample}: \begin{align}\label{eq:kl-intermediate-targets}\mathrm{KL}(\target_{t-1} \| \target_t)=\ln \E_{\target_{t-1}}[\weight_{t-1}\inv(\xt, \xtpo)] - \E_{\target_{t-1}}[\ln \weight_{t-1}\inv(\xt, \xtpo)].\end{align}
%This divergence will be large when a small fraction of particles receive a disproportionately large weight. Otherwise only a small fraction of the particles will receive nontrivial weights, and the rest will be discarded. In that case most particles are discarded, the procedure provides only small effective number of samples and therefore a poor approximation of the target distribution. 

Each step of SMC involves importance sampling of a target $\target_{t-1}$ with $\target_t$ as the proposal, and so the procedure inherits the operating characteristics of importance sampling. Notably this includes an exponential dependence of the number of samples needed for accurate estimation of $\target_{t-1}$ on the Kullback-Leibler divergence of each $\target_t$ from $\target_{t-1}$ \citep{chatterjee2018sample}. In the context of  \Cref{eq:final-target}, we see that $$\mathrm{KL}(\target_{t-1} \| \target_t)=\ln \E_{\target_{t-1}}[\weight_{t-1}\inv(\xt, \xtpo)] - \E_{\target_{t-1}}[\ln \weight_{t-1}\inv(\xt, \xtpo)].$$ This divergence will be large when a small fraction of particles receive a disproportionately large weight.
In that case, only a small fraction of the particles receive nontrivial weights, and the rest will be discarded. Consequently, the procedure provides only small effective number of samples and therefore a poor approximation of the target distribution.
