# Supplementary material for: Practical and Asymptotically Exact Conditional Sampling in Diffusion Models
Source: arXiv:2306.17775 source file (2024-11-23)
Supplement: Supplementary file 2 [file naive_smc.tex]

\section{Naive SMC: importance sampling from unconditional diffusion models}
We here provide details of the naive procedure, showing that it is a case of self-normalized importance sampling.
As mentioned in \Cref{subsec:SMC_framing} importance sampling is a special case of of SMC with a single step (or equivalently several steps, but no resampling at intermediate steps).
It involves a target $\nu$,
and proposal $r$. 
$K$ samples $x_1,\dots, x_K$ are drawn i.i.d.\ from $r$,
and an estimate of $v$ is computed as 
$\hat \nu = \sum w_k x_k$ with each $w_k = \tilde w_k / \sum_k \tilde w_k$
for $\tilde w_k = \nu(x_k)/r(x_k).$
Note hat that the procedure in \Cref{subsec:SMC_framing} is a special case of importance sampling with proposal $r(\dt{x}{0:T})=\pmodel(\dt{x}{0:T})$ and target $\pmodel(\dt{x}{0:T} \mid y)$.
